# Supplementary material for: Observational Learning by Reinforcement Learning
Source: arXiv:1706.06617 source file (2017-06-20)
Supplement: Supplementary file 1 [file appendix.tex]

\section{Appendix A: Baselines}

\subsection{Local view: Baselines for all levels, with (figures in the first column) and without the teacher (second column).}

% \begin{figure}[h]
% \centering
% \foreach \n in {0,32,128}
% \foreach \t in {teacher, noteacher}
% {
% \subfloat{\includegraphics[width=0.49\textwidth]{./figures/local_view/baseline_\t_lstm\n}}
% }
% \hfill
% \caption{Local view: Performance of baselines during training.}
% \end{figure}

% \begin{figure}[h]
% \centering
% \foreach \n in {0,32,64,128}
% \foreach \t in {teacher, noteacher}
% {
% \subfloat{\includegraphics[width=0.49\textwidth]{./figures/local_view/longrun_baseline_\t_lstm\n}}
% }
% \hfill
% \caption{Local view: Performance of baselines during training.}
% \end{figure}

\begin{figure}[h]
\centering
\foreach \n in {0,32,64,128}
\foreach \t in {teacher, noteacher}
{
\subfloat{\includegraphics[width=0.49\textwidth]{./figures/local_view/smooth_longrun_baseline_\t_lstm\n}}
}
\hfill
\caption{Local view: Performance of baselines during training as measured by the average number of steps needed to reach the goal. The results are averaged over 10 random seeds.  }
\end{figure}

\subsection{Global view: Baselines for all levels, with (first column) and without the teacher. (second column)}

\begin{figure}[h]
\centering
\foreach \n in {0,32,64,128}
\foreach \t in {teacher, noteacher}
{
\subfloat{\includegraphics[width=0.49\textwidth]{./figures/global_view/smooth_longrun_baseline_\t_lstm\n}}
}
\hfill
\caption{Global view: Performance of baselines during training. The results are averaged over 10 random seeds. }
\end{figure}
Note, since the goal locations are spread throughout the rooms, the steps need to reach each goal may vary quite a lot depending of the room it is in.  Consequently we opt to smoothen the learning curves, over 25 steps in time, to make the trends in learning easier to read.

\newpage
\section{Appendix B: Videos}
Legend/Colouring used: 
\begin{itemize}
    \item \textbf{Red}: walls in the environment (these are elastic, no effect regeistered when bumping into walls, no negative reward)
    \item \textbf{Black}: background, empty states in the environment
    \item \textbf{Green}: our learning agent/RL agent
    \item [Optional] \textbf{Blue}: teacher/expert agent
    \item [Optional] \textbf{Pink}: active goal in the environment for this episode
\end{itemize}

\subsection{Global view}
All videos show the policy of the agent at the end of training (after training on level 3 -- the 4 rooms scenario):
\begin{itemize}
    \item LAT agent no memory: \texttt{global\_level3\_teacher\_nogoal\_lstm0}
    \item LAT agent with an LSTM(32): \texttt{global\_level3\_teacher\_nogoal\_lstm32}
    \item LAGT agent no memory: \texttt{global\_level3\_teacher\_goal\_lstm0}
    \item LAGT agent with an LSTM(32): \texttt{global\_level3\_teacher\_goal\_lstm32}
\end{itemize}

\subsection{Local view}
All videos show the policy of the agent at the end of training (after training on level 3 -- the 4 rooms scenario):
\begin{itemize}
    \item LAT agent no memory: \texttt{local\_level3\_teacher\_nogoal\_lstm0}
    \item LAT agent with an LSTM(32): \texttt{local\_level3\_teacher\_nogoal\_lstm32}
    \item LAGT agent no memory: \texttt{local\_level3\_teacher\_goal\_lstm0} \\
    \textbf{Observation}: The agent tries to stay close to the teacher and in the instances where it does loose track of it, it either tries to find the teacher or waits for the respawn of the teacher and its next opportunity to follow this agent to the goal
    \item LAGT agent with an LSTM(32): \texttt{local\_level3\_teacher\_goal\_lstm32} \\
    \textbf{Observation}: This agent a bit more independent of the teacher and does not keep as close to the other agent. It remembers the area the teacher was going to, or the door used to exit the room and uses this information to complete the task even if the teacher is not in its vision field anymore. 
\end{itemize}
\subsection{Making the student independent of the teacher}
\begin{itemize}
    \item LAGT agent with local view after being training on all levels with the teacher always present, and the goal always present: \texttt{teacher\_level3\_start}
    \item \textbf{Zero-shot generalization via imitation.} Same agent, but placed in a bigger environment (9 rooms), augmenting the number of goals as well:  \texttt{teacher\_level5\_start}
    \item \textbf{Removing the teacher.} Same agent, but we are not removing the teacher from the environment:  \texttt{noteacher\_level3\_start}
    \item \textbf{After the masking process.} The agent after gradually masking the presence of the teacher:  \texttt{noteacher\_level3\_end}
\end{itemize}

\section{Appendix C: Experimental details}
\subsection{Environment setup}
 The environment will automatically terminate after a maximum of $100$ steps. Agents are given a positive reward of $+1$ when reaching the goal, but no other reward otherwise. When the learning agent reaches the goal, the episode terminates. Note, when the episode terminates, we always re-sample the MDP.
\subsection{Architectures used}
\begin{itemize}
    \item \textbf{Global view experiments}: 2 convolutional layers ((kernel 2x2, stride = 2), (kernel = 2x2, stride = 1)), one fully-connected layer (128 units) + LSTM layer (32 hidden units) for experiments using memory.  
    \item \textbf{Local view experiments}: 1 convolutional layers ((kernel = 2x2, stride = 1)), one fully-connected layer (128 units) + LSTM layer (32 hidden units) for experiments using memory. Note the observational window here is $3$ pixels in all directions around the agent -- a $7x7$ local patch with the agent always in the centered pixel.
\end{itemize}

\end{document}
